# Supplementary material for: Linking evolutionary and ecological theory illuminates non-equilibrium biodiversity
Source: arXiv:1705.04725 ancillary file (2017-05-12)

# Random effect multinomial model

*A. J. Rominger*

*12 May 2017*

## The model

Given the number of sequencing reads assigned to each of  $S$  species, we want to estimate the number of individuals for each species that went into the sequencing run, call that vector  $x$ . We know the total number of reads  $N_{reads}$ , the number of species  $S$ , the total number of individuals  $N$  that were sequenced, and the vector of number of reads per species  $x_{read}$ . We assume that stochastic evolutionary processes have led to some species having a greater propensity to be sequenced. These stochastic processes we summarize in a random effect  $\nu$ . We further assume that within orders these random effects are constant, thus each species within the same order gets the same random effect.

Thus our model for the number of reads is:

$$x_{reads} \sim \text{multinom} \left( N_{reads}, \frac{x\nu}{\sum_i x_i \nu_i} \right)$$

Thus the vector of probabilities for the multinomial distribution is proportional to the unknown abundance times the unknown random effect  $\nu$ .

We could choose to put a multinomial prior on  $x$  because  $N = \sum x$  is fixed, or could approximate  $x_i$  with a continuous prior and assume  $N$  is large enough such that  $Cov(x_i, x_j) \approx 0$ . Allowing  $x_i$  to be iid and continuous allows us to better estimate the relative contribution of  $x$  and  $\nu$  in determining  $x_{reads}$ , so we opt for the prior:

$$\log(x_i) \sim \text{norm} \left( \frac{N}{S}, \sigma_x^2 \right)$$

Given that  $\nu$  is constant within orders, varies across orders, and must be positive, we model it as

$$\log(\nu_{order=j}) \sim \text{norm}(0, \sigma_\nu^2)$$

That is, for order  $j$  the log of the random effect is distributed normally with mean 0 and variance  $\sigma_\nu^2$ .

## Running the model in JAGS

First we set up the simulation

```
# number of orders
n0rd <- 8

# number of species
nspp <- n0rd * 10

# vector identifying which species are in which orders
ordID <- rep(1:n0rd, each = nspp/n0rd)

# simulate random effect
ordSD <- 0.25
set.seed(1)
```

```
ordEffect <- exp(rnorm(nOrd, mean = 0, sd = ordSD))

# generate true abundances for each species
set.seed(1)
x <- sample(seq(1, 80, length.out = nspp))

# simulate number of reads for each species
totReads <- 10^6
set.seed(1)
xreads <- rmultinom(1, totReads, x*ordEffect[ordID])[, 1]
```

A quick plot of what those simulated data look like (colors correspond to order identity)

```
palette(hsv(h = seq(0, 0.8, length.out = max(ordID)),
            s = 1-0.3*seq(-1, 1, length.out = max(ordID))^2,
            v = 0.7 + 0.3*seq(-1, 1, length.out = max(ordID))^2,
            alpha = 0.7))

par(mar = c(3, 3, 0, 0) + 0.5, mgp = c(2, 0.75, 0))
plot(x, xreads, bg = ordID, pch = 21,
     xlab = 'Abundance', ylab = 'Number of reads')
```

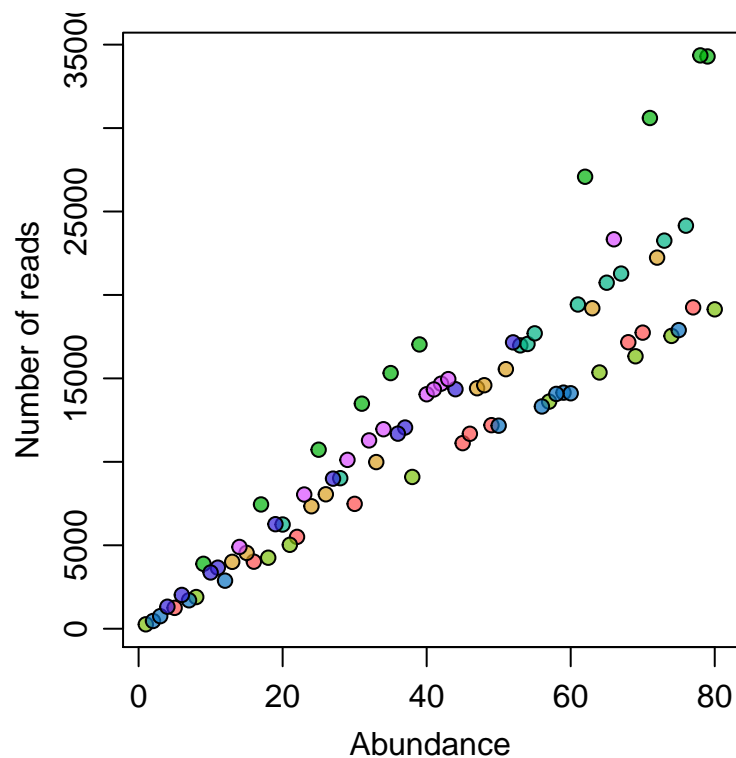

Define the model in JAGS using rjags

```
library(rjags)
```

```
## Loading required package: coda
## Linked to JAGS 4.2.0
## Loaded modules: basemod,bugs
```

```

# write the model out
cat('model{
  # reads model
  xreads[1:S] ~ dmulti(alpha[1:S], totReads)

  # priors
  sigX ~ dunif(0, 100)
  tauX <- 1/(sigX^2)
  sigCopy ~ dunif(0, 100)
  tauCopy <- 1/(sigCopy^2)

  # species-level effect
  for(i in 1:S) {
    logX[i] ~ dnorm(N/S, tauX)
    x[i] <- exp(logX[i])
  }

  # order-level random effect
  for(j in 1:nOrd) {
    logNu[j] ~ dnorm(0, tauCopy)
    nu[j] <- exp(logNu[j])
  }

  # define multinom param
  for(i in 1:S) {
    alpha[i] <- x[i] * nu[ordID[i]]
  }
}',
file = 'multiRandEffect.jag' )

```

Compile the model and configure it for MCMC:

```

# model data and constants
modDat <- list(S = nspp, N = sum(x),
  totReads = totReads, ordID = ordID, nOrd = nOrd,
  # p0 = rep(sum(x)/nspp, nspp),
  xreads = xreads)

## compile model
mod <- jags.model(file = 'multiRandEffect.jag',
  data = modDat,
  n.chains = 1,
  n.adapt = 100)

## Compiling model graph
##   Resolving undeclared variables
##   Allocating nodes
## Graph information:
##   Observed stochastic nodes: 1
##   Unobserved stochastic nodes: 90
##   Total graph size: 385
##
## Initializing model

```

```
# run mcmc
thin <- 10
burn <- 1000
iter <- 5000
samp <- coda.samples(mod,
                      var = c('sigCopy', 'x', 'logNu'),
                      n.iter = (iter + burn) * thin,
                      thin = thin)
samp <- as.matrix(samp[[1]])[-(1:burn), ]
```

Now plot real versus estimated abundance. Error bars are 95% credible intervals, red line is 1:1 line:

```
xest <- sum(x) * samp[, grep('x', colnames(samp))] /
  rowSums(samp[, grep('x', colnames(samp))])
xestCI <- apply(xest, 2, quantile, prob = c(0.025, 0.975))

par(mar = c(3, 3, 0, 0) + 0.5, mgp = c(2, 0.75, 0))
plot(x, colMeans(xest), cex = 0.5,
     panel.first = {
       segments(x0 = x, y0 = xestCI[1, ], y1 = xestCI[2, ])
       points(x, colMeans(xest), col = 'white', pch = 16, cex = 0.5)
     },
     ylim = range(xestCI),
     xlab = 'Actual abundance', ylab = 'Estimated abundance')
abline(0, 1, col = 'red')
```

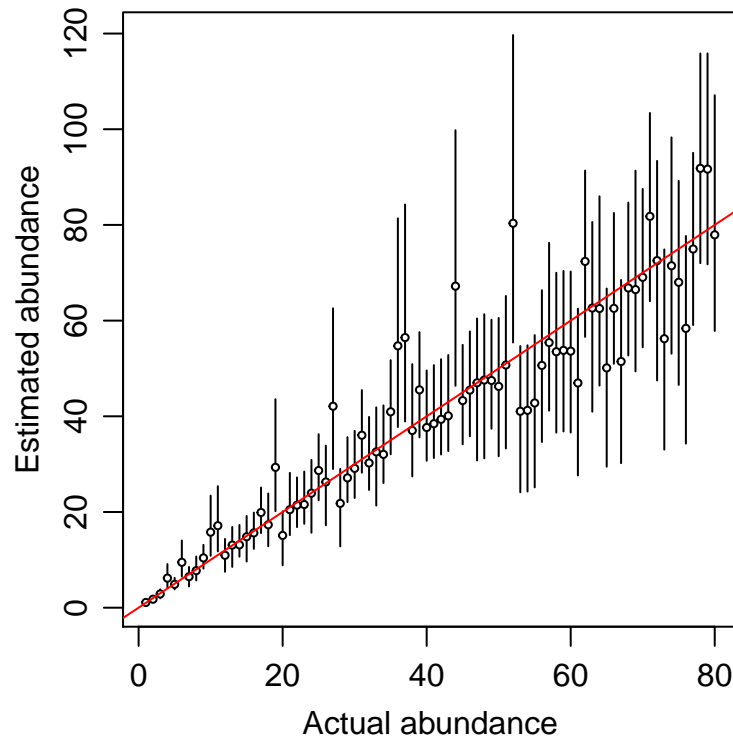

Plot  $\sigma_{order}$ , red line is true value:

```
par(mar = c(3, 3, 0, 0) + 0.5, mgp = c(2, 0.75, 0))
plot(samp[, 'sigCopy'], type = 'l',
     xlab = 'Iterations', ylab = expression(sigma[orders]))
```

```
abline(h = ordSD, col = 'red')
```

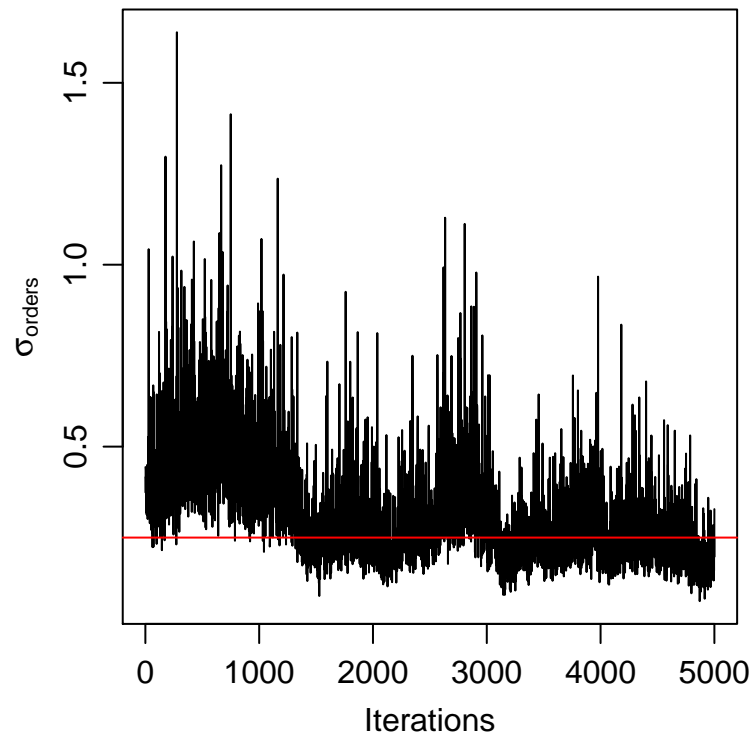

Supplement: Supplementary file 1 [file modelDerivation_normPrior.pdf]
